# Supplementary material for: On Tradeoffs in Learning-Augmented Algorithms
Source: arXiv:2501.12770 source file (2025-01-22)
Supplement: Supplementary file 2 [file appendix2.tex]

\section{Smooth Algorithm for One-Max Search}

\subsection{Proof of Lemma \ref{lem:OM-case1-smooth}}

\subsection{Proof of Lemma \ref{lem:OM-case2-smooth}}

\subsection{Proof of Proposition \ref{prop:OM-brittle}}
