# Supplementary material for: On Tradeoffs in Learning-Augmented Algorithms
Source: arXiv:2501.12770 source file (2025-01-22)
Supplement: Supplementary file 3 [file appendix3.tex]

\section{Average-Case Analysis in Ski-Rental}

\subsection{Proof of Theorem \ref{thm:sr-smoothness}}

\subsection{Proof of Theorem \ref{thm:sr-avg}}

\subsection{Proof of Corollary \ref{cor:sr-avg}}
